# Supplementary material for: Dual theory of transmission line outages
Source: arXiv:1606.07276 ancillary file (2017-01-22)
Supplement: Supplementary file 1 [file supplement.pdf]

# Dual theory of transmission line outages — Supplemental material

Henrik Ronellenfitsch,* Debsankha Manik,† Jonas Hörsch,
Tom Brown,‡ Dirk Witthaut§

January 21, 2017

## 1 Computational performance of the dual method

In this section of the supplement, we show the full comparison between the computation time of the conventional and the dual method for the calculation of LODFs.

### 1.1 Computing LODFs

Conventionally, the line outage distributions factors (LODFs) are calculated from power transfer distribution factors (PTDFs) via the formula

$$\mathrm{LODF}_{k\ell} = \frac{[\mathbf{PTDF} \cdot \boldsymbol{K}]_{k\ell}}{1 - [\mathbf{PTDF} \cdot \boldsymbol{K}]_{\ell\ell}}\,, \tag{1}$$

where $\boldsymbol{K}$ is the node-edge incidence matrix. The PTDF matrix is given by

$$\mathbf{PTDF} = \boldsymbol{B}_d \boldsymbol{K}^t \boldsymbol{B}^*. \tag{2}$$

where $\boldsymbol{B}_d \in \mathbb{R}^{L \times L}$ is the diagonal matrix of line susceptances and the asterisk denotes the Moore-Penrose pseudo-inverse. The computationally most demanding part is the inversion of the matrix $\boldsymbol{B} = \boldsymbol{K}\boldsymbol{B}_d\boldsymbol{K}^t$. In practical applications one usually does not compute the full pseudo-inverse $\boldsymbol{B}^*$, but instead solves the linear system of equations

$$\mathbf{PTDF} \cdot \boldsymbol{B} = \boldsymbol{B}_d \boldsymbol{K}^t. \tag{3}$$

*H. R. is at the Department of Physics and Astronomy, University of Pennsylvania.

†H. R. and D. M. are at the Max Planck Institute for Dynamics and Self-Organization (MPIDS), 37077 Göttingen, Germany.

‡J. H. and T. B. are at the Frankfurt Institute for Advanced Study, 60438 Frankfurt am Main, Germany.

§D. W. is at the Forschungszentrum Jülich, Institute for Energy and Climate Research - Systems Analysis and Technology Evaluation (IEK-STE), 52428 Jülich, Germany and the Institute for Theoretical Physics, University of Cologne, 50937 Köln, Germany.

```
tic;
PTDF = zeros(L,N);
Bf = Bd * K';
B = K * Bf;
PTDF(:,an) = Bf(:,an) / B(an,an);
PTDF = full(PTDF * K);
LODF = PTDF./(ones(L,L)-ones(L,1)*diag(PTDF)');
LODF = LODF-diag(diag(LODF))-eye(L,L);
toc

tic;
TEMP = C * full((C' * Xd * C) \ C');
LODFdual = -TEMP./(ones(L,1)*diag(TEMP)');
toc
```

Figure 1: Matlab code to compare the runtime of the conventional algorithm and the dual method. All variable names are same as those used in the text with the exception of `an`, which indexes all nodes except for the slack.

In addition one usually excludes the slack node $s$ from the calculation, i.e. one deletes the $s$th row and column of the matrix $\boldsymbol{B}$ and the $s$th column of the matrix $\mathbf{PTDF}$ and the matrix $\boldsymbol{B}_d\boldsymbol{K}^t$. This approach is implemented for instance in the popular software package MATPOWER 5.1 [3]. A program code in Matlab for the calculation of a matrix containing all LODFs using this approach is listed in Figure 1.

The dual approach can significantly speed up the calculation of the LODFs when the power grid is not too heavily meshed. In particular, the LODFs are given by

$$\mathrm{LODF}_{k,\ell} = -\frac{\boldsymbol{u}_k^t \boldsymbol{C}\boldsymbol{A}^{-1}\boldsymbol{C}^t\boldsymbol{u}_\ell}{\boldsymbol{u}_\ell^t \boldsymbol{C}\boldsymbol{A}^{-1}\boldsymbol{C}^t\boldsymbol{u}_\ell}\,. \tag{4}$$

with the matrix

$$\boldsymbol{A} = \boldsymbol{C}^t\boldsymbol{X}_d\boldsymbol{C}. \tag{5}$$

In practice we do not calculate the full inverse of the matrix $\boldsymbol{A}$, but solve the linear system of equations

$$\boldsymbol{A}\cdot\mathbf{TEMP'} = \boldsymbol{C}^t \tag{6}$$

and set $\mathbf{TEMP} = \boldsymbol{C}\cdot\mathbf{TEMP'}$. The LODFs (4) are then simply given by

$$\mathrm{LODF}_{k,\ell} = \frac{\mathbf{TEMP}_{k,\ell}}{\mathbf{TEMP}_{\ell,\ell}}. \tag{7}$$

A program code in Matlab for the calculation of a matrix containing all LODFs in this way is listed in Figure 1.

Table 1: Comparison of CPU time for the calculation of the PTDFs obtained with the MATLAB code listed in Fig. 1.

| Test Grid | | Grid Size | | | | CPU time in seconds | | speedup |
|---|---|---|---|---|---|---|---|---|
| name | source | nodes $N$ | lines $L$ | cycles $L-N+1$ | cycles/nodes $\frac{L-N+1}{N}$ | Conventional method | Dual method | $t_{\text{conv}}/t_{\text{dual}}$ |
| sparse numerics: | | | | | | | | |
| case300 | [3] | 300 | 409 | 110 | 0.37 | $0.009 \pm 0.002$ | $0.005 \pm 0.001$ | 1.83 |
| case1354pegase | [2] | 1354 | 1710 | 357 | 0.26 | $0.217 \pm 0.011$ | $0.049 \pm 0.002$ | 4.43 |
| GBnetwork | [1] | 2224 | 2804 | 581 | 0.26 | $0.59 \pm 0.02$ | $0.14 \pm 0.01$ | 4.09 |
| case2383wp | [3] | 2383 | 2886 | 504 | 0.21 | $0.67 \pm 0.03$ | $0.16 \pm 0.02$ | 4.20 |
| case2736sp | [3] | 2736 | 3495 | 760 | 0.28 | $0.95 \pm 0.06$ | $0.29 \pm 0.04$ | 3.27 |
| case2746wp | [3] | 2746 | 3505 | 760 | 0.28 | $0.96 \pm 0.06$ | $0.29 \pm 0.03$ | 3.35 |
| case2869pegase | [2] | 2869 | 3968 | 1100 | 0.38 | $1.13 \pm 0.09$ | $0.40 \pm 0.05$ | 2.79 |
| case3012wp | [3] | 3012 | 3566 | 555 | 0.18 | $1.02 \pm 0.07$ | $0.26 \pm 0.03$ | 3.93 |
| case3120sp | [3] | 3120 | 3684 | 565 | 0.18 | $1.10 \pm 0.07$ | $0.28 \pm 0.04$ | 3.96 |
| case9241pegase | [2] | 9241 | 14207 | 4967 | 0.54 | $15.5 \pm 0.8$ | $11.9 \pm 0.4$ | 1.31 |
| dense numerics: | | | | | | | | |
| case300 | [3] | 300 | 409 | 110 | 0.37 | $0.012 \pm 0.002$ | $0.005 \pm 0.001$ | 2.68 |
| case1354pegase | [2] | 1354 | 1710 | 357 | 0.26 | $0.498 \pm 0.014$ | $0.107 \pm 0.006$ | 4.65 |
| GBnetwork | [1] | 2224 | 2804 | 581 | 0.26 | $1.82 \pm 0.05$ | $0.36 \pm 0.01$ | 5.06 |
| case2383wp | [3] | 2383 | 2886 | 504 | 0.21 | $2.09 \pm 0.06$ | $0.33 \pm 0.01$ | 6.26 |
| case2736sp | [3] | 2736 | 3495 | 760 | 0.28 | $3.34 \pm 0.13$ | $0.67 \pm 0.05$ | 4.97 |
| case2746wp | [3] | 2746 | 3505 | 760 | 0.28 | $3.34 \pm 0.11$ | $0.68 \pm 0.05$ | 4.94 |
| case2869pegase | [2] | 2869 | 3968 | 1100 | 0.38 | $4.19 \pm 0.08$ | $1.20 \pm 0.02$ | 3.49 |
| case3012wp | [3] | 3012 | 3566 | 555 | 0.18 | $3.88 \pm 0.13$ | $0.53 \pm 0.03$ | 7.30 |
| case3120sp | [3] | 3120 | 3684 | 565 | 0.18 | $4.23 \pm 0.11$ | $0.56 \pm 0.01$ | 7.54 |
| case9241pegase | [2] | 9241 | 14207 | 4967 | 0.54 | $135.4 \pm 1.4$ | $58.6 \pm 0.5$ | 2.31 |

All input matrices appearing in the calculations exhibit a sparse structure (i.e. they contain many identically zero entries). Hence it is sensible to use specialized sparse numerical algorithms to compute the LODFs. In MATLAB this is achieved by converting all input matrices appearing in the code of Fig. 1 into the sparse format using the command `sparse`. MATLAB then employs the high-performance supernodal sparse Cholesky decomposition solver CHOLMOD 1.7.0 for the solution of the linear system of equations. The resulting LODF matrix is full (i.e., it usually contains no zeros), such that we convert the results back to a full matrix using the command `full`. Care has to be taken for the dual method about where to do the conversion (see the code example in Fig. 1).

## 1.2 Comparison of CPU time

Many real-world power grids are only weakly meshed such that the number of fundamental cycles $L - N + 1$ is much smaller than the number of nodes $N$. Hence, the matrix $\boldsymbol{A} \in \mathbb{R}^{(L-N+1)\times(L-N+1)}$ is significantly smaller than the matrix $\boldsymbol{B} \in \mathbb{R}^{N\times N}$ appearing in the conventional approach. Hence the dual method is significantly faster in many cases of practical relevance.

We have tested the computation time using the the MATLAB code listed in Figure 1. The CPU times of both the conventional and the dual method are evaluated using the commands `tic` and `toc` for a variety of test grids from [1–3]. The results are listed in Table 1 using both dense and sparse numerical algorithms. We observe that the dual method is faster by a factor of 1.31 to 4.43

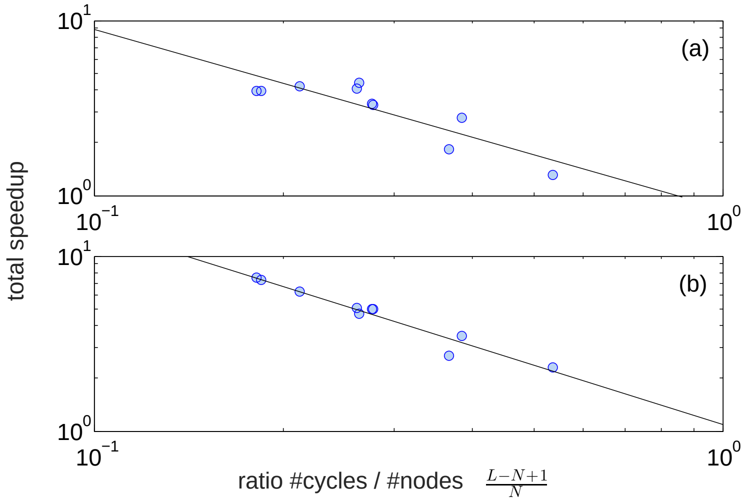


Figure 2: Depending on network topology, the dual method can significantly speed up the calculation of the LODFs. We show the ratio of the runtimes of the conventional node-based method and the dual method as a function of the ratio of the numbers of cycles $L - N + 1$ and the number of nodes $N$ for the test grids described in Table 1 for (a) specialized sparse numerics and (b) standard dense numerics. The black line is a power law fit $a \times [(L - N + 1)/N]^{-\gamma}$ to the data, which yields the parameters (a) $\alpha = 1.0214$ and $\gamma = 0.8452$ for the sparse numerics, and (b) $\alpha = 1.0864$ and $\gamma = 1.1303$ for the dense numerics.

when using sparse numerics. The speed-up is even higher when using standard dense numerics, ranging between 2.31 and and 7.54 for the test grids under consideration.

In Figure 2, we show plots of speedup against the ratio of the number of cycles $L - N + 1$ and number of nodes $N$ in the network as well as a power law fit to the data.

# 2 Formal proofs

In this section, we provide the formal proofs for the propositions in the main paper.

## 2.1 Proof of Proposition 2

*Proof.* If there is only one independent path between two vertex sets, then by the definition of vertex-independence, all paths between the two vertex sets must share at least one common vertex, the 'bridge'. The existence of the bridge allows the definition of two sub-graphs, each of which contains one of the vertex sets but which share only the bridge vertex in common. Each sub-graph

consists of the union of all paths between each vertex set and the bridge that only contain the bridge once.

The existence of the bridge partitions the cycles into two sets, corresponding to the cycles of the two sub-graphs. The cycles on either side of the bridge cannot share any edge with a cycle from the other side of the bridge, since the sub-graphs share only the bridge in common. If we write the matrix $\boldsymbol{A} = \boldsymbol{C}^t \boldsymbol{X}_d \boldsymbol{C}$ in components,

$$A_{cc'} = \begin{cases} \sum_{\ell \in \kappa_c} x_\ell & \text{if } c = c'; \\ \sum_{\ell \in \kappa_c \cap \kappa_{c'}} \pm x_\ell & \text{if } c \neq c, \end{cases} \tag{8}$$

where $\kappa_c$ is the set of edges in the cycle $c$, we see that $\boldsymbol{A}$ becomes block diagonal for the two sets of cycles. The LODF defined in (4) inherits this block diagonal structure, since $\boldsymbol{A}^{-1}$ is also block diagonal, and therefore the LODF must vanish for edges from different sets. □

## 2.2 Proof of Proposition 3

In the following we analyze the solution of equation

$$\boldsymbol{A}\, \Delta \boldsymbol{f} = \boldsymbol{q} \tag{9}$$

with $\boldsymbol{q} = F_\ell(\boldsymbol{u}_\ell^t \boldsymbol{C} \boldsymbol{A}^{-1} \boldsymbol{C}^t \boldsymbol{u}_\ell)^{-1} \boldsymbol{C}^t \boldsymbol{u}_\ell$ and $\boldsymbol{A} = \boldsymbol{C}^t \boldsymbol{X}_d \boldsymbol{C}$. for plane graphs. W.l.o.g. we assume that both the original network and the dual graph are connected. Otherwise we can just focus on the connected component which includes the perturbed edge resp. the perturbed cycles and exclude all disconnected parts from our analysis.

**Definition 1.** *A positive domain $\mathcal{D}_+$ is a connected subgraph of the dual with $\Delta f_c \geq 0$ for all $c \in \mathcal{D}_+$ and at least one cycle with $\Delta f_c > 0$. The domain $\mathcal{D}_+$ is called isolated if $\Delta f_d \leq 0$ for all cycles $d$ in the immediate neighborhood of the domain $\mathcal{D}_+$. Analogously we use $\mathcal{D}_-$ for a domain with opposite signs.*

**Definition 2.** *We denote by $\mathcal{B}$ the set of edges which form the boundary of the graph, i.e. the set of edges which is adjacent to only one cycle in the dual graph:*

$$\mathcal{B} = \left\{ \ell \in E \,\middle|\, \sum_c C_{\ell,c} \neq 0 \right\}. \tag{10}$$

If $\ell \notin \mathcal{B}$ then it belongs to exactly two faces. As we have fixed the orientation of all faces to be counter-clockwise we then have

$$\sum_{\text{cycles } b} C_{\ell,b} = 0. \tag{11}$$

If $\ell \in \mathcal{B}$ then it belongs to exactly one cycle $c'$. Thus we have

$$\sum_{\text{cycles } b} C_{\ell,b} C_{\ell,c} = C_{\ell,c}^2 = \begin{cases} 1 & \text{if } c = c' \\ 0 & \text{if } c \neq c'. \end{cases} \tag{12}$$

**Lemma 1.** *Each isolated domain $\mathcal{D}_+$ must contain a cycle $c_1$ with $q_{c_1} > 0$ and each isolated domain $\mathcal{D}_-$ must contain a cycle $c_2$ with $q_{c_2} < 0$.*

*Proof.* To prove this statement assume the opposite: Let $\mathcal{D}'$ be a domain with $\Delta f_c \geq 0$ and $q_c \leq 0$ for all $c \in \mathcal{D}'$ and at least one cycle with $\Delta f_c > 0$. Using equation (9) we find that

$$\begin{aligned}\sum_{c\in\mathcal{D}'} A_{cc}\Delta f_c &= -\sum_{c\in\mathcal{D}'}\sum_{d\neq c} A_{cd}\Delta f_d + \sum_{c\in\mathcal{D}'} q_c \\ &= -\sum_{c\in\mathcal{D}'}\sum_{\substack{d\in\mathcal{D}'\\ d\neq c}} A_{cd}\Delta f_d - \sum_{c\in\mathcal{D}'}\sum_{d\notin\mathcal{D}'} A_{cd}\Delta f_d \\ &\quad + \sum_{c\in\mathcal{D}'} q_c. \end{aligned} \tag{13}$$

Furthermore, using the definition (5) of the matrix $A$, we have

$$\begin{aligned}\sum_{\text{cycles}\, d} A_{dc} &= \sum_{\text{cycles}\, d}\sum_{\text{edges}\ell} C_{\ell,d}C_{\ell,c}x_\ell \\ &= \sum_{\ell\notin\mathcal{B}} \underbrace{\sum_{\text{cycles}\, d} C_{\ell,d}}_{=0} C_{\ell,c}x_\ell + \sum_{\ell\in\mathcal{B}} \underbrace{\sum_{\text{cycles}\, d} C_{\ell,d}C_{\ell,c}}_{=C_{\ell,c}^2} x_\ell\,. \end{aligned} \tag{14}$$

Thus we have

$$A_{cc} = -\sum_{d\neq c} A_{dc} + \sum_{\ell\in\mathcal{B}} C_{\ell,c}^2 x_\ell \tag{15}$$

such that

$$\begin{aligned}\sum_{c\in\mathcal{D}'} A_{cc}\Delta f_c &= -\sum_{c\in\mathcal{D}'}\sum_{\substack{d\in\mathcal{D}'\\ d\neq c}} A_{dc}\Delta f_c - \sum_{c\in\mathcal{D}'}\sum_{d\notin\mathcal{D}'} A_{dc}\Delta f_c \\ &\quad + \sum_{c\in\mathcal{D}'}\sum_{\ell\in\mathcal{B}} C_{\ell,c}^2\, x_\ell. \end{aligned} \tag{16}$$

Comparing the two expressions (14) and (16) and using the symmetry $A_{cd} = A_{dc}$ we find that

$$\begin{aligned} &-\sum_{c\in\mathcal{D}'}\sum_{d\notin\mathcal{D}'} A_{cd}\Delta f_d + \sum_{c\in\mathcal{D}'} q_c \\ &= -\sum_{c\in\mathcal{D}'}\sum_{d\notin\mathcal{D}'} A_{dc}\Delta f_c + \sum_{c\in\mathcal{D}'}\sum_{\ell\in\mathcal{B}} C_{\ell,c}^2\, x_\ell. \end{aligned} \tag{17}$$

Using the facts that $A_{cd} \leq 0$ for all $c \neq d$ and $\Delta f_d \leq 0$ for all cycles $d$ in the immediate neighborhood of the isolated domain $\mathcal{D}'$, we find that the left-hand side of this equation is smaller or equal to zero. On the contrary we have $\Delta f_c \geq 0$ for all cycles $c \in \mathcal{D}'$ and $\Delta f_c > 0$ for at least one cycle $c \in \mathcal{D}'$ such that the right-hand side is strictly larger than zero. This leads to a contradiction such that the assumption must be wrong and no such domain $\mathcal{D}'$ exists. □

**Corollary 1.** *Consider the solution of equation (9) if exactly one edge $\ell$ fails.*

*If the edge $\ell$ lies in the interior of the graph ($\ell \notin \mathcal{B}$), then we have $q_{c_1} > 0$ and $q_{c_2} = -q_{c_1} < 0$ for the two cycles $c_1, c_2$ adjacent to the edge $\ell$ and $q_c = 0$ otherwise. Then $\mathcal{D}_+$ contains the cycle $c_1$ and $\mathcal{D}_-$ contains the cycle $c_2$ and no further isolated domains can exist.*

*If the edge $\ell$ lies on the boundary of the graph ($\ell \in \mathcal{B}$), then only a single cycle $c_1$ is affected with $q_{c_1} \neq 0$. Hence there is only one domain in the graph such that $\Delta f_c \geq 0$ for all cycles $c$ if $q_{c_1} > 0$ and $\Delta f_c \leq 0$ for all cycles $c$ if $q_{c_1} < 0$.*

## 2.3 Proof of Proposition 4

As before we analyze the solution of equation (9) and assume that both the original network and the dual graph are connected. In the following we denote by $\text{dist}(c, c')$ the graph theoretic distance of two vertices $c$ and $c'$ of the dual graph.

**Definition 3.** *We denote by $u_d$ ($\ell_d$) the maximum (minimum) value of cycle flows $\Delta f_c$ for all vertices $c$ of the dual graph with a given distance $d$ to a reference vertex $c'$:*

$$
\begin{aligned}
u_d &= \max_{c, \text{dist}(c,c')=d} \Delta f_c \\
\ell_d &= \min_{c, \text{dist}(c,c')=d} \Delta f_c .
\end{aligned}
\tag{18}
$$

**Lemma 2.** *The maximum value of the cycle flows $u_d$ decreases monotonically with the distance to the reference cycle $c' = c_1$ for which $q_{c_1} > 0$:*

$$
u_d \leq u_{d-1}, \qquad 1 \leq d \leq d_{\max}. \tag{19}
$$

*The minimum $\ell_d$ increases monotonically with the distance to the reference cycle $c' = c_2$ for which $q_{c_2} < 0$:*

$$
\ell_d \geq \ell_{d-1}, \qquad 1 \leq d \leq d_{\max}. \tag{20}
$$

*Proof.* The proof is carried out by induction starting from $d = d_{\max}$. We only give the proof for the maximum, the proof for the minimum proceeds in an analogous way. We assume that the network is large enough such that $d_{\max} \geq 2$, otherwise the statement is trivial anyway.

(1) Base case $d = d_{\max}$: Consider the vertex $c$ of the dual for which $\text{dist}(c, c_1) = d_{\max}$ and $\Delta f_c$ assumes its maximum $\Delta f_c = u_{d_{\max}}$. By assumption we have $\text{dist}(c, c_1) \geq 2$ such that the face $c$ cannot be adjacent to the

pertured edge such that $q_c = 0$. Equation (9) yields

$$\begin{aligned} A_{cc}\Delta f_c &= -\sum_{b\neq c} A_{cb}\Delta f_b \\ &= -\sum_{\substack{b\neq c \\ \mathrm{dist}(b,c_1)=d_{\max}}} A_{cb}\Delta f_b + \sum_{\substack{b\neq c \\ \mathrm{dist}(b,c_1)=d_{\max}-1}} A_{cb}\Delta f_b. \end{aligned} \tag{21}$$

We define the abbreviations

$$\mathcal{A}_d = -\sum_{b\neq c, \mathrm{dist}(b,c_1)=d} A_{cb} \tag{22}$$

and use some important properties of the matrix $A$:

$$\begin{aligned} & A_{cb} \leq 0 \text{ for } c \neq b \qquad \Rightarrow \qquad \mathcal{A}_d \geq 0 \\ & A_{cc} \geq \mathcal{A}_{d_{\max}} + \mathcal{A}_{d_{\max}-1} \,. \end{aligned} \tag{23}$$

We can furthermore bound the values of $\Delta f_b$ in equation (21) by $u_{d_{\max}}$ or $u_{d_{\max}-1}$, respectively, such that we obtain

$$\begin{aligned} u_{d_{\max}} = \Delta f_c &\leq \frac{\mathcal{A}_{d_{\max}} u_{d_{\max}} + \mathcal{A}_{d_{\max}-1} u_{d_{\max}-1}}{\mathcal{A}_{d_{\max}} + \mathcal{A}_{d_{\max}-1}} \\ \Rightarrow \; u_{d_{\max}} &\leq u_{d_{\max}-1}, \end{aligned} \tag{24}$$

(2) Inductive step $d \to d-1$: We consider the vertex $c$ of the dual graph with $\mathrm{dist}(c, c_1) = d$ and $\Delta f_c = u_d$. Staring from equation (9) and using the same estimations as above, we obtain

$$\begin{aligned} u_d = \Delta f_c &= \frac{q_c - \sum_{b\neq c} A_{cb}\Delta f_b}{A_{cc}} \\ &\leq \frac{\mathcal{A}_{d-1} u_{d-1} + \mathcal{A}_d u_d + \mathcal{A}_{d+1} u_{d+1}}{\mathcal{A}_{d-1} + \mathcal{A}_d + \mathcal{A}_{d+1}} \,. \end{aligned} \tag{25}$$

Note that the inhomogeneity $q_c \leq 0$ for all vertices except for $c = c_1$. With the induction hypothesis $u_{d+1} \leq u_d$ this yields

$$\begin{aligned} u_d &\leq \frac{\mathcal{A}_{d-1} u_{d-1} + (\mathcal{A}_d + \mathcal{A}_{d+1}) u_d}{\mathcal{A}_{d-1} + \mathcal{A}_d + \mathcal{A}_{d+1}} \\ \Rightarrow u_d &\leq u_{d-1}. \end{aligned} \tag{26}$$

which completes the proof. □

**Lemma 3.** *The maximum (minimum) value of the cycle flows $u_d$ decreases (increases)* strictly *monotonically with the distance to the reference cycle $c_1$*

*($c_2$)*

$$u_d < u_{d-1},$$
$$\ell_d > \ell_{d-1}, \qquad 1 \le d \le d_{\max}. \tag{27}$$

*if (1) all cycles $c$ at maximum distance from $c_1$ lie at the boundary of the dual graph,*

$$\forall c \,\text{with}\, \text{dist}(c, c_1) = d_{\max} : \tag{28}$$
$$\exists \,\text{edge}\, \ell \,\text{with}\, \ell \in \mathcal{B} \,\text{and}\, C_{\ell,c} \neq 0. \tag{29}$$

*or (2) all extrema $u_d$ and $\ell_d$ are unique.*

*Proof.* We show that in both cases we can replace $\ge$ by $>$ in the base case and thus also in the inductive step in the proof of lemma 2. If condition (1) is satisfied we have

$$A_{cc} > \mathcal{A}_{d_{\max}} + \mathcal{A}_{d_{\max}-1} \tag{30}$$

due to boundary terms. If condition (1) is not satisfied but condition (2) is, then the sum in equation (21) includes at least two terms. One of the values of $\Delta f_b$ in the sum must be strictly smaller than the maximum value $u_d$ or $u_{d-1}$, respectively, as we assumed that these maxima are unique. We thus can replace the $\ge$ by $>$ in the estimations. □

# 3 Decay in regular lattices

In this section we analytically calculate the cycle flows induced by a line outage for a uniform regular square lattice in the the continuum limit. Consider a network with cycle edge adjacency matrix $C_{\ell,c}$. Then we are interested in a continuous version of equation (9) , written in components

$$\sum_{d=1}^{L-N+1} A_{cd} \Delta f_d = q_c. \tag{31}$$

On a square lattice, the application of $A_{cd}$ to a vector in the bulk can be written, going to the continuous limit (see Fig. 3),

$$(A\phi)(x) = \frac{\phi(x,y)}{B(x+h/2,y)} + \frac{\phi(x,y)}{B(x-h/2,y)} \tag{32}$$
$$+ \frac{\phi(x,y)}{B(x,y+h/2)} + \frac{\phi(x,y)}{B(x,y-h/2)} \tag{33}$$
$$- \frac{\phi(x+h,y)}{B(x+h/2,y)} - \frac{\phi(x-h,y)}{B(x-h/2,y)} \tag{34}$$
$$- \frac{\phi(x,y+h)}{B(x,y+h/2)} - \frac{\phi(x,y-h)}{B(x,y-h/2)} \tag{35}$$
$$= h^2 \nabla \cdot \left( \frac{1}{B(x,y)} \nabla \phi \right) + O(h^3). \tag{36}$$

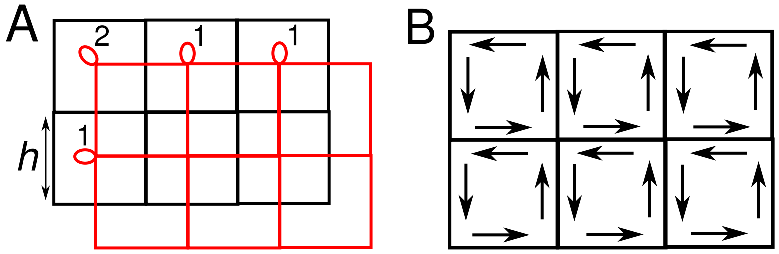


Figure 3: A. A square lattice (black) together with its cycle-dual (red). The cycle dual is also a square lattice, but because the boundary edges are only adjacent to one cycle, it contains self-loops at its boundary nodes. The weight of a self loop is the sum of all boundary edge weights which are part of the boundary cycle. In the limit $h \to 0$, the self-loops enforce Dirichlet boundary conditions on the cycle density, $\phi|_{\partial A} = 0$. B. Consistently oriented cycles in a square lattice.

Here, $h$ is the lattice spacing and $B(x, y)$ is the (continuous) line susceptance. The right hand side works similarly, noting that only two cycles contribute, with opposite signs. Let us assume that the failing line $\ell$ is parallel to the $y$ axis and situated at the origin. Then the RHS is

$$= h^2 \frac{\partial}{\partial x} \left( F_y(0,0) \frac{q_{c_1}}{B(0,0)(B(0,0) - q_{c_1})} \delta^{(2)}(x, y) \right) + O(h^3). \tag{37}$$

This is a dipole source field with dipole moment parallel to the $x$ axis. It is easy to see the generalization to arbitrary dipole moments. Thus, the full continuous equations governing the behavior of the cycle density in the bulk are

$$\nabla \cdot \left( \frac{1}{B} \nabla \phi \right) = -\boldsymbol{p} \cdot \nabla \delta^{(2)}(\boldsymbol{x} - \boldsymbol{a}), \tag{38}$$

for a perturbation at $\boldsymbol{a}$. The dipole vector $\boldsymbol{p}$ is orthogonal in direction to flow at the site of perturbation and proportional to it in magnitude. More perturbations can be handled by linear combination.

At the boundary, a similar relation as in the bulk holds, supplying us with boundary conditions. Because boundary cycles possess three neighboring cycles

but four edges in total, some terms are left over:

$$(A\phi)(x) = \frac{\phi(x,y)}{B(x+h/2,y)} + \frac{\phi(x,y)}{B(x-h/2,y)} \tag{39}$$

$$+ \frac{\phi(x,y)}{B(x,y+h/2)} + \frac{\phi(x,y)}{B(x,y-h/2)} \tag{40}$$

$$- \frac{\phi(x+h,y)}{B(x+h/2,y)} - \frac{\phi(x-h,y)}{B(x-h/2,y)} \tag{41}$$

$$- \frac{\phi(x,y-h)}{B(x,y-h/2)} \tag{42}$$

$$= \frac{\phi(x,y)}{B(x,y)} + O(h). \tag{43}$$

Thus, we find that Dirichlet boundary conditions must hold in the absence of boundary perturbations: $\phi|_{\partial A} = 0$.

Finally, we need a law telling us how to calculate a flow vector $\Delta \boldsymbol{F}(\boldsymbol{x})$ from the cycle density. To this end, consider Figure 3 B. In order to obtain the $y$ component of a flow vector, we need to add up the contributions of two cycle flows neighboring in the $x$ direction, and vice versa. Thus, the flow vector becomes

$$\Delta \boldsymbol{F}(\boldsymbol{x}) = \begin{pmatrix} \phi(x,y+h/2) - \phi(x,y-h/2) \\ \phi(x-h/2,y) - \phi(x+h/2,y) \end{pmatrix} \tag{44}$$

$$\sim \begin{pmatrix} 0 & 1 \\ -1 & 0 \end{pmatrix} \nabla\phi. \tag{45}$$

In the case of uniform susceptance $B(x,y) \equiv B$, equation (38) becomes a regular Poisson equation in two dimensions with dipole source density. The solutions to this equation are well known from the theory of electrostatics, on an infinite domain taking the form

$$\phi(\boldsymbol{x}) = \frac{\boldsymbol{p}\cdot\boldsymbol{x}}{\boldsymbol{x}^2} \tag{46}$$

$$\Delta \boldsymbol{F}(\boldsymbol{x}) = \begin{pmatrix} 0 & 1 \\ -1 & 0 \end{pmatrix} \left( \frac{\boldsymbol{p}}{\boldsymbol{x}^2} - 2\boldsymbol{x}\frac{\boldsymbol{p}\cdot\boldsymbol{x}}{\boldsymbol{x}^4} \right) \tag{47}$$

for a perturbation at $\boldsymbol{a} = 0$.

# 4 Decomposing cycle flows in general networks and Proof of Proposition 5

There is a directed connected graph $G = (V, E)$. It has $|E| - |V| + 1$ independent cycles.

Choose a non-crossing embedding of the graph $G$ on an orientable, closed, connected two-dimensional manifold $\Sigma$ (i.e. a Riemann surface), such that the

surface has the minimum genus $g$ such that the graph can be drawn without crossing. This is the genus $g$ of the graph.

The embedding partitions the surface into a set of faces (each face is homeomorphic to a disk and contractible on the surface) $F$, which we choose to be oriented all the same way. $\cup F = \Sigma$. At each edge exactly two faces meet and this edge is oppositely oriented in each face.

We now have a 2d cell complex $(F, E, V)$ with chain groups $G_i$ generated over $\mathbb{Z}$

$$G_F \overset{\delta_2 = \tilde{C}}{\rightarrow} G_E \overset{\delta_1 = K}{\rightarrow} G_V \tag{48}$$

and boundary operators $\tilde{C}, K$ satisfying $\delta_1 \delta_2 = K\tilde{C} = 0$.

We also have cohomology spaces $\Omega_i(\Sigma)$ with exterior derivatives $d_i$ given by

$$\Omega_0(\Sigma) \overset{d_0 = BK^t}{\rightarrow} \Omega_1(\Sigma) \overset{d_1 = \tilde{C}^t X}{\rightarrow} \Omega_2(\Sigma) \tag{49}$$

Note that the derivatives satisfy $d_1 d_0 = \tilde{C}^t X B K^t = \tilde{C}^t K^t = 0$.

The Euler characteristic is given by

$$\chi(\Sigma) = 2 - 2g = |F| - |E| + |V| \tag{50}$$

The boundaries of the faces define a set of $|F|$ oriented cycles $\tilde{C}$, only $|F| - 1$ of which are independent.

In addition there is a set of $2g$ independent topological cycles $\hat{C}$ which are non-contractible and provide a basis of the first homology group $H_1(\Sigma, \mathbb{Z}) = \mathbb{Z}^{\otimes 2g}$ (since the definition of the homology group is cycles modulo boundaries).

Together $\tilde{C}$ and $\hat{C}$ span all the cycles $C$ of the graph

$$|C| = |\tilde{C}| + |\hat{C}| = |F| + 2g = |E| - |V| + 2 \tag{51}$$

If one of the face-boundaries is removed, the cycles become independent and form a basis of the cycles.

The choice of boundary cycles $\tilde{C}$ is fixed by the embedding. We choose the basis of $\hat{C}$ to span the elements of $\ker(K)$ which are orthogonal to $\tilde{C}$ with respect to the norm defined by the diagonal matrix $X$ of always-positive series reactances. In equations we have

$$\tilde{C}^t X \hat{C} = \hat{C}^t X \tilde{C} = 0 \tag{52}$$

(This definition guarantees that each element of $\hat{C}$ cannot be a linear combination of $\tilde{C}$ and therefore is an element of the homology: if $\hat{C} = \tilde{C} Z$ for some matrix $Z$, then $0 = \hat{C}^t X \tilde{C} = Z^t \tilde{C}^t X \tilde{C}$ which implies $Z = 0$.)

With this choice we now return to the central equation of the LODF paper. If we consider all the cycles $C = (\tilde{C}, \hat{C})$ then we have for a line outage on line $\ell$:

$$C^t X C \Delta f \propto C^t u_\ell \tag{53}$$

This decomposes into two equations, where we can now make use of eq. (52):

$$\tilde{C}^t X C \Delta f = \tilde{C}^t X \tilde{C} \Delta \tilde{f} + \tilde{C}^t X \hat{C} \Delta \hat{f} = \tilde{C}^t X \tilde{C} \Delta \tilde{f} \propto \tilde{C}^t u_\ell \tag{54}$$

$$\hat{C}^t X C \Delta f = \hat{C}^t X \tilde{C} \Delta \tilde{f} + \hat{C}^t X \hat{C} \Delta \hat{f} = \hat{C}^t X \hat{C} \Delta \hat{f} \propto \hat{C}^t u_\ell \tag{55}$$

where $\Delta\tilde{f}$ and $\Delta\hat{f}$ are the changed cycle flows on the boundary and topological cycles respectively.

If we consider the first equation:

$$\tilde{C}^t X \tilde{C} \Delta\tilde{f} \propto \tilde{C}^t u_\ell \tag{56}$$

this is identical with the planar case: the matrix $\tilde{C}$ is the sparse incidence matrix of the dual graph, $\tilde{C}^t X \tilde{C}$ is the Laplacian of the dual graph and $\tilde{C}^t u_\ell$ is a dipole, because at each edge only two faces meet, oppositely oriented.

The second equation has no simple interpretation:

$$\hat{C}^t X \hat{C} \Delta\hat{f} \propto \hat{C}^t u_\ell \tag{57}$$

On the RHS, $\hat{C}^t$ is dense (i.e. a linear combination of nearly all edges) so cannot be described as some localised multi-pole. Similarly the LHS is also a dense matrix with no interpretation as e.g. a Laplacian.

So to summarise: the effects of a line outage on the cycle flows $\Delta f$ can be in general be decomposed into two parts: a dipole effect on the cycles which define boundaries of faces, which decays monotonically; a non-local complicated interaction, which only affects the flows on the topological cycles $\hat{C}^t$, but impacts nearly all the edges.

# References


[1] W. A. Bukhsh and Ken McKinnon. Network data of real transmission networks. `http://www.maths.ed.ac.uk/optenergy/NetworkData/`, 2013. [Online; accessed 03-August-2015].

[2] S. Fliscounakis, P. Panciatici, F. Capitanescu, and L. Wehenkel. Contingency ranking with respect to overloads in very large power systems taking into account uncertainty, preventive and corrective actions. *IEEE Trans. Power Syst.*, 28:4909, 2013.

[3] R. D. Zimmerman, C. E. Murillo-Sanchez, and R. J. Thomas. Matpower: Steady-state operations, planning and analysis tools for power systems research and education. *IEEE Trans. Power Syst.*, 26:12, 2011.
